# Supplementary material for: RynnVLA-001: Using Human Demonstrations to Improve Robot Manipulation
Source: arXiv:2509.15212 source file (2025-09-18)
Supplement: Supplementary file 1 [file appendix.tex]

% \newpage
\appendix
Appendix.
